# Supplementary material for: Capillary rupture of suspended polymer concentric rings
Source: arXiv:1502.03207 ancillary file (2015-02-11)
Supplement: Supplementary file 1 [file Supplementary.pdf]

# Supplementary for "Capillary rupture of suspended polymer concentric rings"


Zheng Zhang,[1] G.C. Hilton,[2] Ronggui Yang,[1] and Yifu Ding[1, 3,*]

[1]*Department of Mechanical Engineering, University of Colorado at Boulder, Boulder, Colorado 80309, USA*
[2]*National Institute of Standards and Technology, Boulder, Colorado 80305, USA*
[3]*Materials Science and Engineering Program, University of Colorado at Boulder, Boulder, Colorado 80309, USA*

*Correspondence: yifu.ding@colorado.edu


## 1. Experimental details

Polystyrene "PS35k" (Average molecular weight $M_w$ ≈35 kg/mol, as determined with GPC; Glass transition temperature $T_g$= 95 ℃) was purchased from Sigma-Aldrich Co. LLC. Poly(methyl methacrylate) "PMMA15k" (Average $M_w$ ≈ 15 kg/mol, as determined with GPC; $T_g$= 88 ℃) was purchased from Scientific Polymer Products, Inc. Both polymers were used as received.

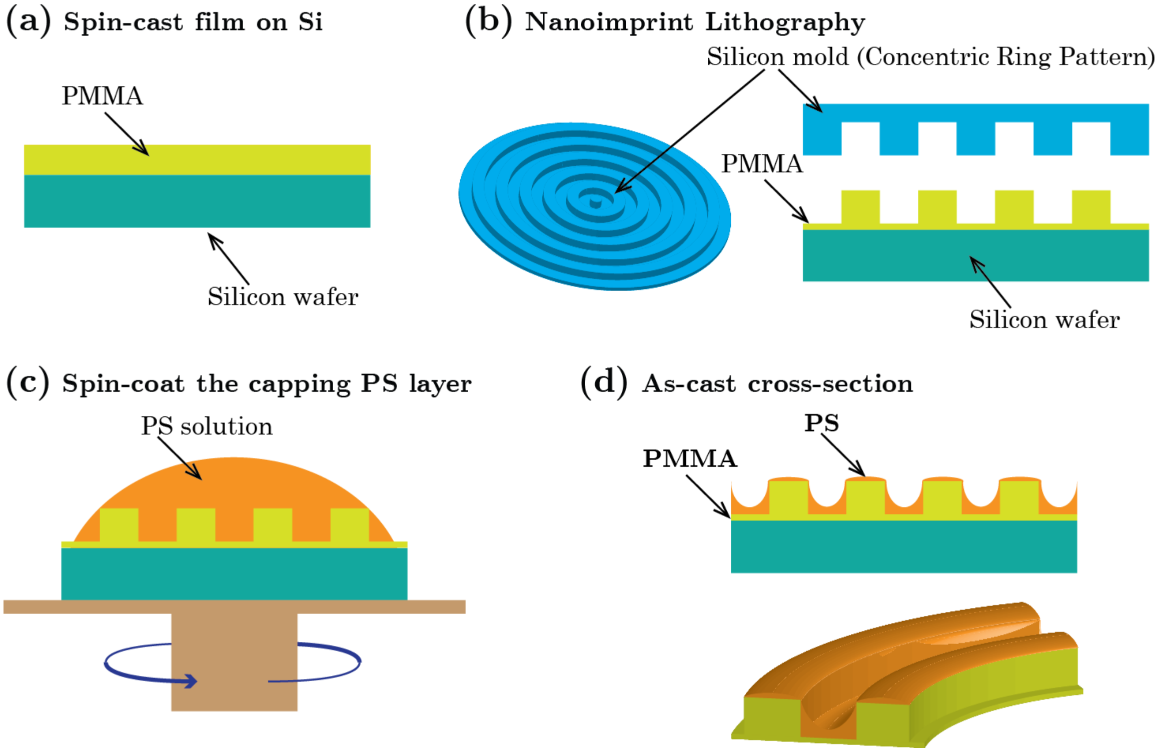


*Figure S1 Fabrication procedure for the concentric pattern*

PMMA15k films were first spin-coated onto silicon wafers at 2000 rpm, from a 20 wt% solution in toluene (Fig. S1(a)). Prior to use, the wafers had been cleaned with oxygen plasma. The thickness of the film was determined from the step height measurement of a razor blade scratch, using atomic force microscopy (AFM, Dimension 3100, Bruker Corporation). We used Gwyddion for AFM image analysis.

An Eitre 3 nanoimprinter (Obducat, Inc.) was used to replicate micron-scale concentric ring patterns from a rigid silicon mold onto the PMMA films. The mold was fabricated via a standard Si micromachining protocol: exposing the photoresist on wafer with a standard *i*-line wafer stepper and etching the Si using DRIE (deep reactive ion etcher) via "Bosch process". The pattern was replicated via the thermal-embossing mode of nanoimprint lithography (NIL), at 160 ℃ temperature and 4 MPa normal pressure for 20 minutes (Fig. S1(b)).

Subsequently, PS35k was spin-coated onto the PMMA pattern from an 8 wt% solvent in 1-chloropentane, a selective solvent for PS which would not deteriorate the bottom PMMA pattern during spin-coating (Fig. S1(c)). The bilayer films were then annealed *in vacuo* at 50 ℃ (below the $T_g$ of PMMA) for 8 hours in order to remove residual solvent.

We then anneal the bilayer films at 170 ℃ on an STC200 microscopy hot-stage (Instec, Inc., temperature stability ±0.1 ℃). The instabilities of the surface structures were observed in-situ with an Olympus BX60 optical microscope, while the sample was being annealed at constant temperature. ImageJ was used to process the power spectrum density profiles, extract the average capillary wavelengths and calculate surface areas occupied by each phase.

# 2. Supplementary figures

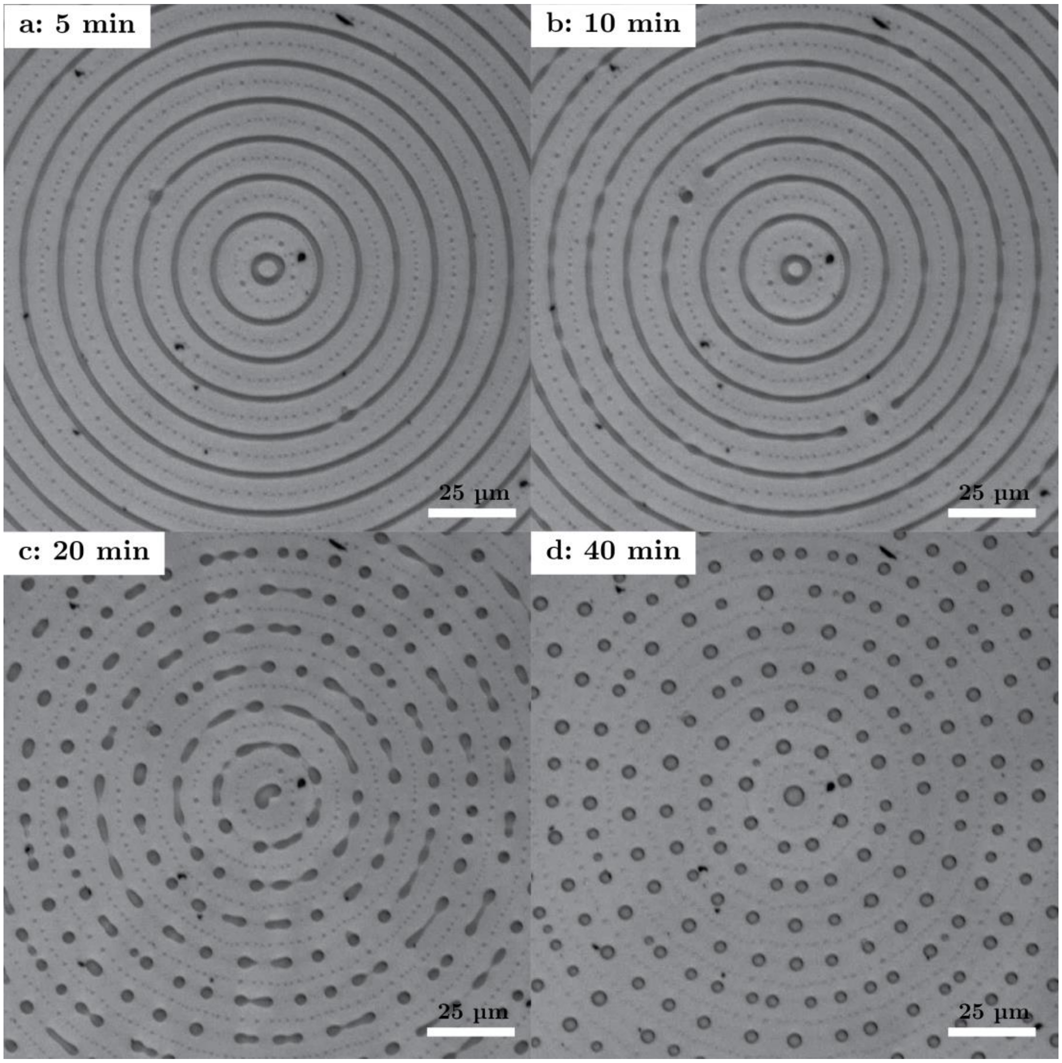


*Figure S2 Optical snapshots of "Sample A" annealed at 160 °C for the labeled duration.*

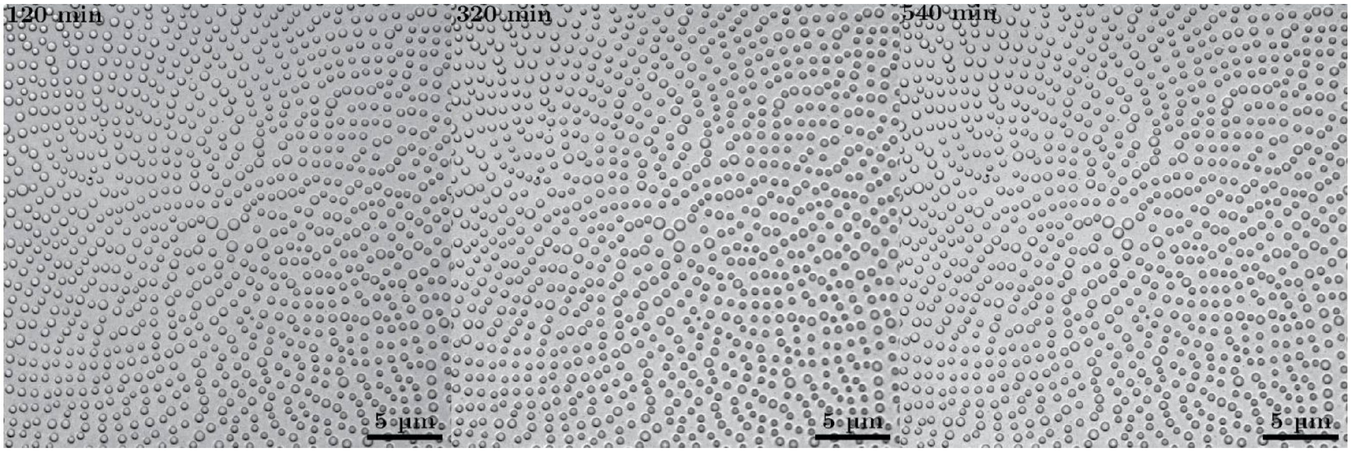


*Figure S3 Optical snapshots of "Sample B" annealed at 170 °C for the labeled duration.*

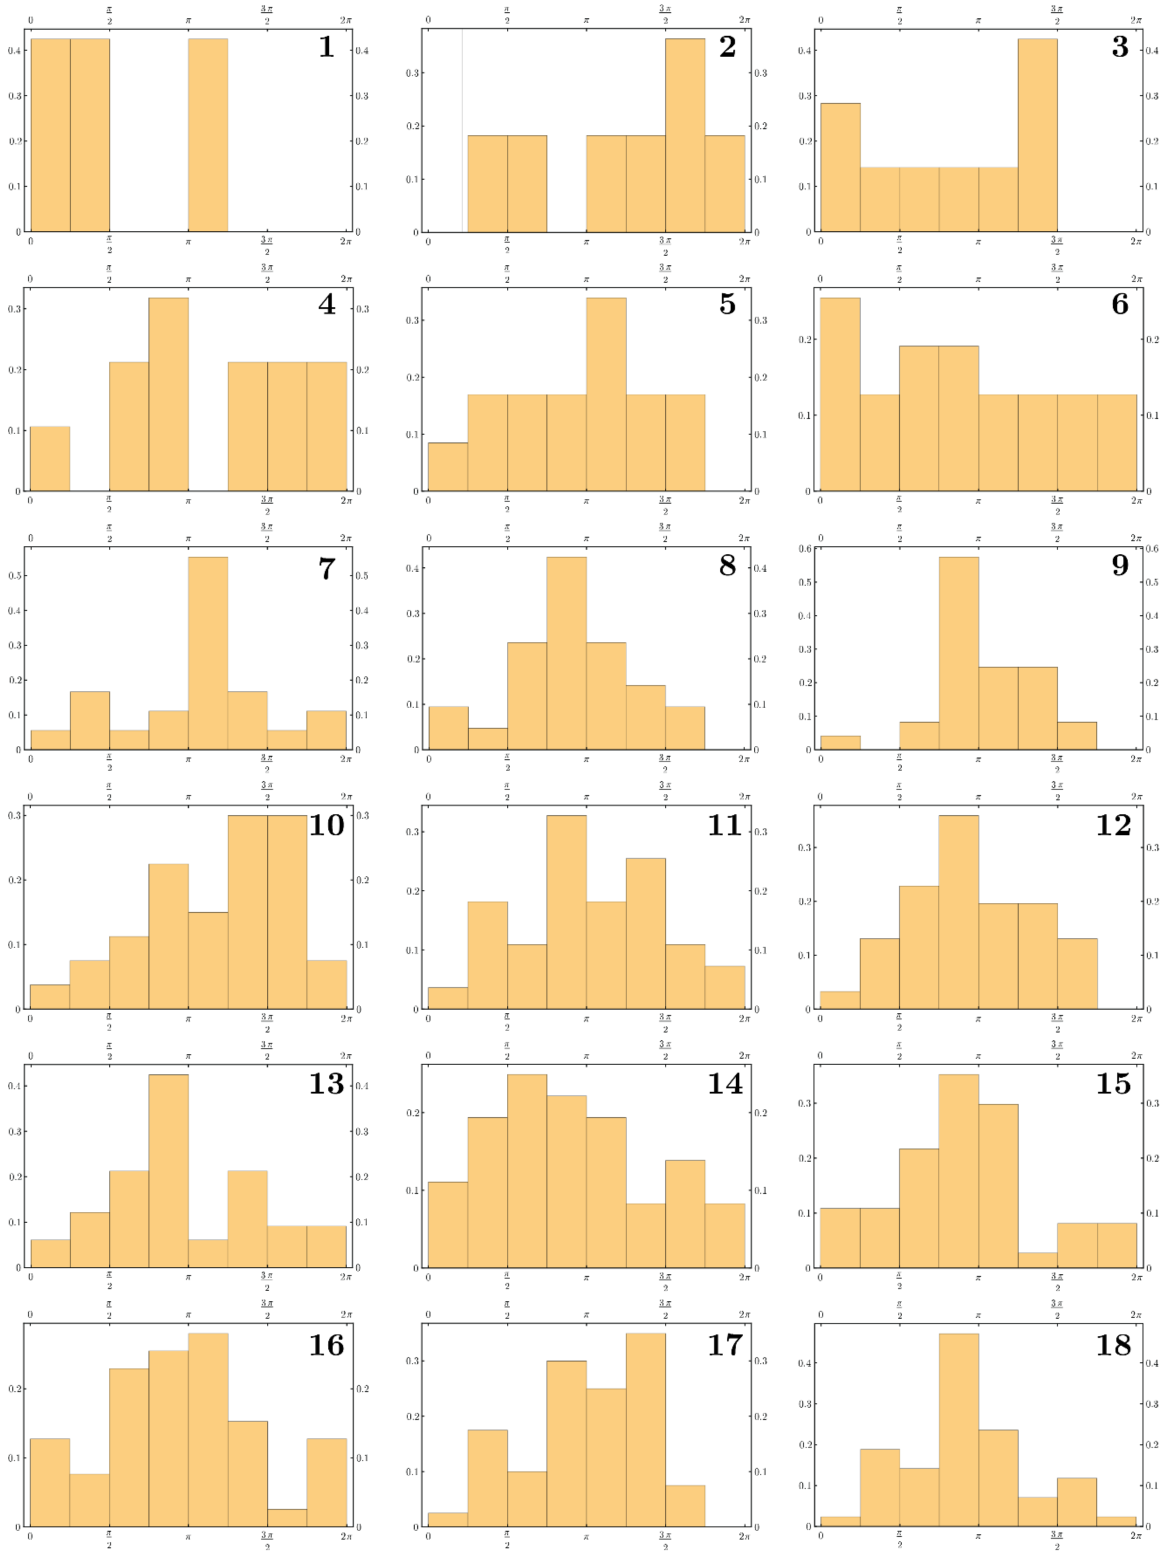


*Figure S4 Distribution of $\phi$ for each PS ring in Sample B. X-axis is $\phi$. Y-axis is probability.*

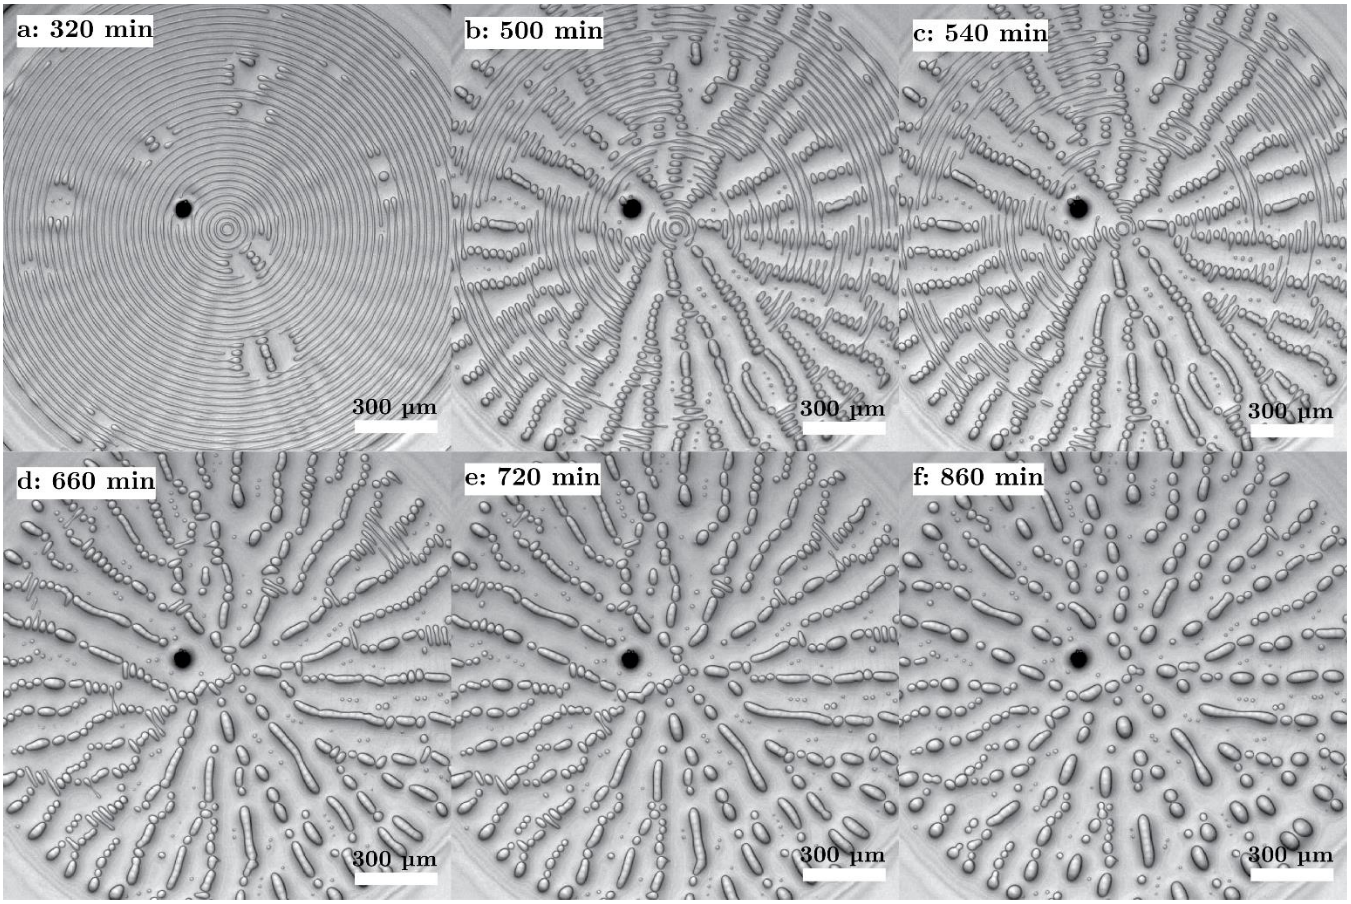

*Figure S5 Optical snapshots of "Sample C" annealed at 170 °C for the labeled duration.*

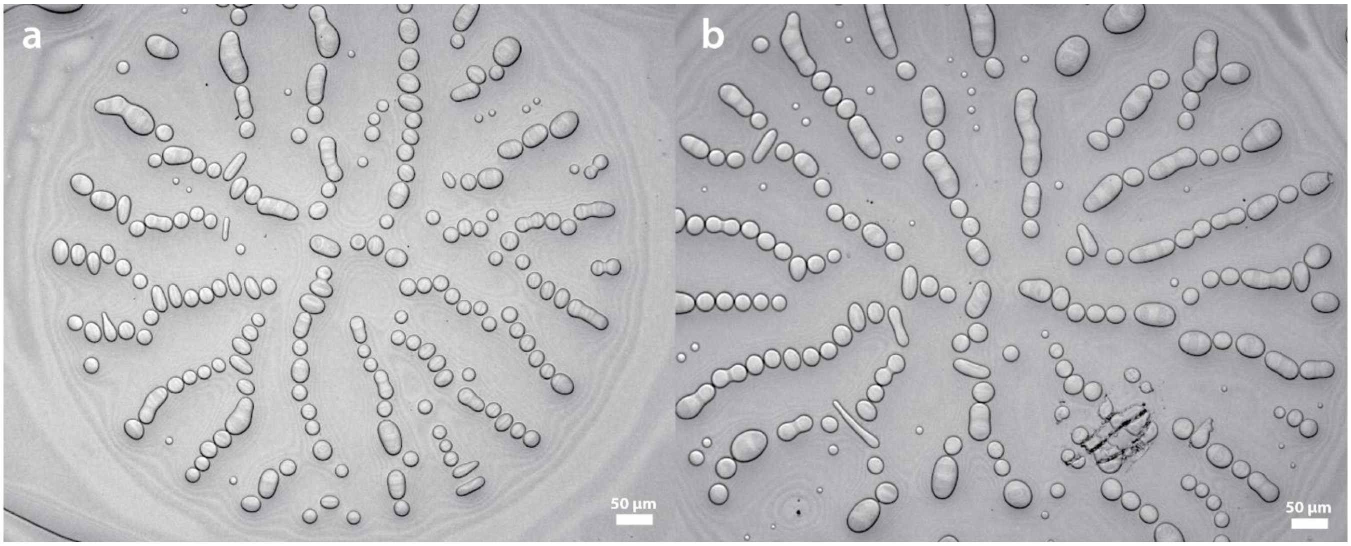

*Figure S6 Optical image of other strongly confined ($H/h < 1.3$) samples, annealed at 170°C for 860 min.*

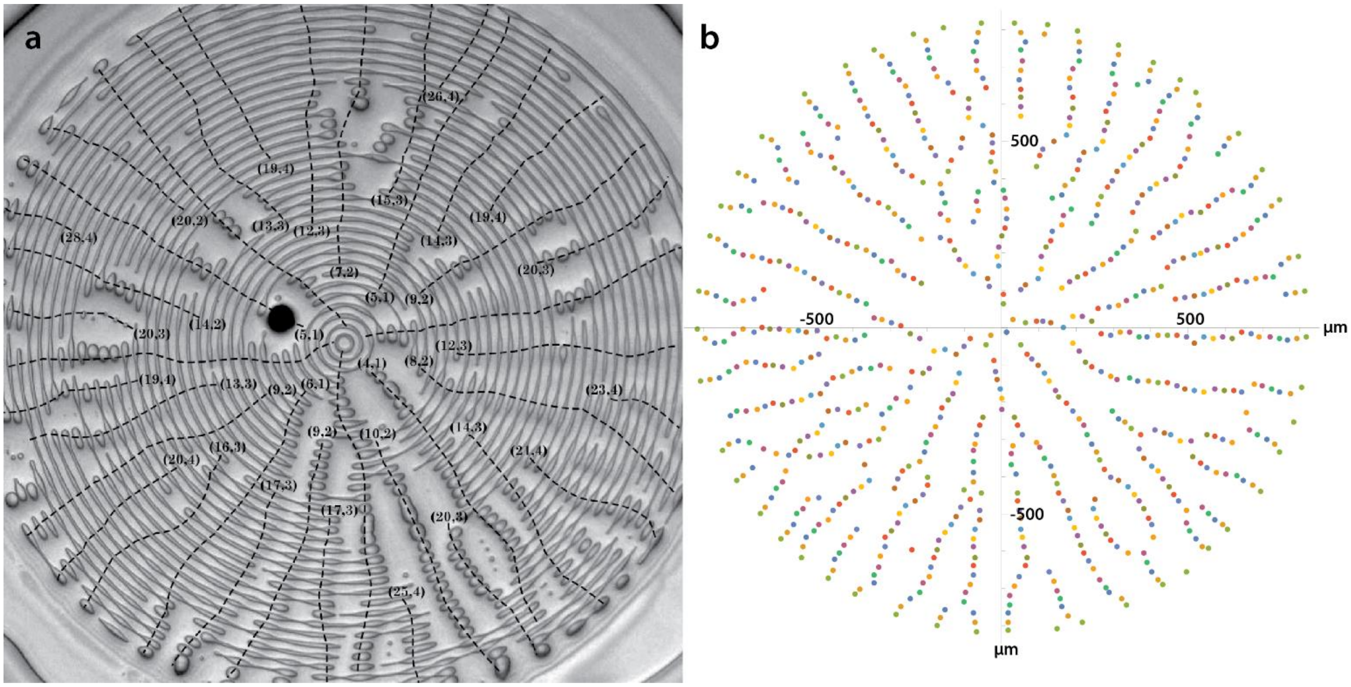


*Figure S7 (a) Illustration of the inserted new waves on the optical image of Sample C annealed at 170 °C for 420 min. Each new insertion is denoted by (x, n), where x is the order of the ring and n is the order of the generation. (b) The corresponding digitized coordinated of the fluctuation peaks.*
